# Supplementary material for: $k$-Universality of Regular Languages
Source: arXiv:2311.10658 source file (2023-11-17)
Supplement: Supplementary file 1 [file appendixproofs.tex]

\ifpaper
\noindent
{\textbf{Lemma~\ref{lem:direct_paths_sufficent_every_word}.}
     Every path recognised by  an NFA $\mathcal{A}$ is $k$-universal iff every simple accepting path in it is $k$-universal.
\begin{proof}
	% Assume first, that every word recognised by $\mathcal{A}$ is $k$-subsequence universal. 
	% Note that there must exist at least one non-cyclic path in $\mathcal{A}$. % Thus by assumption the words associated with the paths are $k$-subsequence universal as such the paths.
	% For the other direction, assume that every non-cyclic accepting path is $k$-subsequence universal. 
	In one direction, if $\mathcal{A}$ accepts any path that is not $k$-universal,  then not every path recognised by $\mathcal{A}$ is $k$-universal.
	Otherwise,  the set of paths induced by every word recognised by $\mathcal{A}$ must contain, as a subsequence, some non-cyclic path.
	Therefore, if each non-cyclic path is $k$-universal, then every path is.
	% Since, every word induced by a non-cyclic accepting path is $k$-subsequence universal, then every word recognised by $\mathcal{A}$ is $k$-subsequence universal.
\end{proof}
\else
\fi

\ifpaper
\bigskip
\noindent
{\textbf{Lemma~\ref{lem:reaching_every_state_further}.}
Let $q, q' \in Q$ be a pair of states in the NFA $\mathcal{A}$ such that there exists a path $\pi$ from $q$ to $q'$ where the final transition in $\pi$ is labelled $\tx \in \Sigma$.
    Then, there exists some path $\pi'$ of length at most $n$ from $q$ to $q'$ where the final transition in the path is labelled $\tx$.
\input{proofs/reaching_every_state_further.tex}
\else
\fi

\ifpaper
\bigskip
\noindent
\textbf{Lemma~\ref{lem:ksu_min_length}.}
	For an NFA $\mathcal{A}$ with $n$ states, if there is a $k$-universal word recognised by $\mathcal A$, then there is a $k$-universal word recognised by $\mathcal{A}$ of length at most $ kn\sigma - (n-1)(k-1)$. 
\input{proofs/ksu_min_length.tex}
\else
\fi

\ifpaper
\bigskip
\noindent
\textbf{Lemma~\ref{lem:ESUPFA}.}
For a given an NFA $\mathcal{A}$ with $n$ states and $|\Sigma|=\sigma$, we can decide in $O(n^3 \sigma 2^\sigma)$ time whether $\mathcal{A}$ accepts words whose universality index is arbitrarily large. If the answer is negative, then we can compute the largest universality index of a word accepted by $\mathcal{A}$. 
\input{proofs/lem-esupfa}
\else
\fi

%\ifpaper
%\bigskip
%\noindent
%\textbf{Theorem~\ref{thm:ESUPFA}.}
%For a given NFA $\mathcal{A}$ with $n$ states and $|\Sigma|=\sigma$ and a natural number $k\in\N$, $k$-ESU is decidable in $O(n^3 \sigma^2 2^\sigma)$ time.
%\input{proofs/thm-esupfa}
%\else
%\fi

\ifpaper
\bigskip
\noindent
\textbf{Lemma~\ref{lem:ASUPFA}.}
For a given an NFA $\mathcal{A}$ with $n$ states and $|\Sigma|=\sigma$, we can compute in $O(n^3 \sigma 2^\sigma)$ time the smallest universality index of a word accepted by $\mathcal{A}$. 
\begin{proof}
Clearly, the set of words accepted by $\mathcal{A}$ which have the smallest universality index (among all words accepted by $\mathcal{A}$) includes a word which is the label of a simple path in $\mathcal{A}$. So, to solve the problem stated in this lemma it is enough to consider only words which are the label of simple paths in $\mathcal{A}$. The length of these words is upper bounded by $n$. This also shows that their universality index is upper bound by $n$ (so, as a consequence, this universality index and the numbers smaller than it fit in one memory word). 

	The solution of our problem is done by a dynamic programming algorithm. We define two $n\times 2^\sigma$ matrices $M, M'$ where initially $M[q][V]=M'[q][V]=\infty$ for $V\subseteq \Sigma$. Also, we use a set $L=\emptyset$. Further, set $M[q_0][\emptyset]=0$ and insert $(q_0,\emptyset)$ in $L$.
	
	We will maintain the property that before the \nth{$(r+1)$} iteration of our algorithm (for $r\geq 0$) $M[q][S]$ stores the minimal number of arches of the word $w_{r,q}$ of length at most $r$ which connects $q_0$ and $q$ such that $\letters(\r(w_{r,q})) = S$. This property clearly holds before the first iteration of the algorithm. 
	Now, we perform the following steps
\begin{lstlisting}[mathescape=true,backgroundcolor = \color{white}]
for $\ell = 1$ to $n$
  for all $(q,S) \in L$ 
    for all $a\in \Sigma$ and $q'\in \delta(q,\ta)$
      if $S\cup \{\ta\}=\Sigma$
        set $M'[q'][\emptyset]=M[q][S]+1$ and insert $(q',\emptyset)$ in $L$
      else 
        set $M'[q'][S\cup\{\ta\}]=M[q][S]$ and insert $(q',S\cup\{\ta\})$ in $L$
for all $q \in Q$ and $V\subseteq \Sigma$
  set $M[q][V]=\min\{M[q][V],M'[q][V]\}$
\end{lstlisting}
% 	\begin{algorithmic}
% 	\For{$\ell = 1$ to $n$}
% 		\ForAll{$(q,S) \in L$} 
% 			\ForAll{$a\in \Sigma$ and $q'\in \delta(q,\ta)$}
% 				\If{$S\cup \{\ta\}=\Sigma$}
% 					\State set $M'[q'][\emptyset]=M[q][S]+1$ and insert $(q',\emptyset)$ in $L$
% 				\Else 
% 					\State set $M'[q'][S\cup\{\ta\}]=M[q][S]$ and insert $(q',S\cup\{\ta\})$ in $L$
% 				\EndIf 
% 			\EndFor
% 		\EndFor
% 	\EndFor
% 	\ForAll{$q \in Q$ and $V\subseteq \Sigma$}
% 		\State set $M[q][V]=\min\{M[q][V],M'[q][V]\}$
% 	\EndFor
% 	\end{algorithmic}
% 	
	In the iteration of the outmost for-loop for $\ell=r$ we actually consider, for each pair $(q,S)$, the word $v$ of length at most $r-1$ which connects $q_0$ and $q$, such that $v$ has a minimum number of arches and $\letters(\r(v)) = S$ (the relevant information about this path, i.e., its rest and the number of arches is stored in $M$), and try to extend this path by one letter $\ta$. This leads to another pair $(q',S\cup\{\ta\})$, and we simply check if this is the word $v'$ with a minimum number of arches, of length at most $r$ which connects $q_0$ and $q'$, such that $\letters(\r(v'))$ is either $\emptyset$, when $\Sigma = S\cup\{\ta\}$, or $S\cup\{\ta\}$ otherwise (see also Lemma \ref{lem:making_a_path_longer}, which explains how a path is extended). This implies that the property which we wanted to maintain holds before the iteration of the loop for $\ell=r+1$. 
	
	The time complexity of this algorithm is $ O^*(n^3 2^\sigma)$.
	
	Now, the smallest universality index of a word accepted by $\mathcal{A}$ is simply the minimum entry $M[q][V]$, for a final state $q$.
\end{proof}

\else
\fi

%\ifpaper
%\bigskip
%\noindent
%\textbf{Theorem~\ref{thm:ASUPFA}.}
%$k$-ASU, for an input automaton $\mathcal{A}$ with $n$ states, and input alphabet of size $\sigma$, and a natural number $k$, is decidable in $\mathcal{O}(n^3\sigma 2^\sigma)$ time.
%\input{proofs/thm-asupfa}
%\ifpaper
%\else
%\fi

\ifpaper
\bigskip

Next, we present a full version of the NP-hardness of $k$-ESU.

\medskip

\noindent
\textbf{Theorem~\ref{thm:NP_hard_1_universal}.}
$k$-ESU is NP-hard.
\begin{proof}
	Let $G = (V, E)$ be a graph with $V = \{v_1, v_2, \dots, v_n\}$.
	
	An automaton $\mathcal{A}$ is constructed from $G$  as follows over the alphabet $\Sigma = \{1, 2, \dots n\}$. 
	Let $Q = \{q_{i,j} \mid i,j \in [n]\} \cup \{q_0, q_f\}$ where the last two states indicate the initial state and a failure state. The set of accepting states is given by $F = \{q_{n,j} \mid j \in [n]\}$.
	% Informally, the state $q_{i,j}$ is used to represent visiting vertex $v_j$ at the $i^{th}$ step of some path. 
	Now, we define the transition function $\delta : Q \times \Sigma \to Q$ by 
	\begin{align*}
		\delta(q, x) = 
		\begin{cases} 
			q_{i+1,\ell}, & \text{if } q = q_{i,j}, x = \ell, i < n, \text{ and } (v_j,v_\ell) \in E,\\
			q_f, & \text{if }  q=q_{i,j}\text{ and } (v_j,v_x) \not\in E,\\
			q_{1,x}, & \text{if } q = q_0,\\
			q_f & \text{if } q = q_{n, i}.
		\end{cases}
	\end{align*}
	Thus, the set of transition from each state $q_{i,j}$ represents the edges in $G$ incident to $v_j$. Each transition is labelled by the end vertex of the edge, i.e., the vertex that is reached after following the edge. Since $\mathcal{A}$ has $n^2+2$ states, $\mathcal{A}$ is constructible in polynomial time.

	%\bigskip
	
	Using this construction, observe that any word accepted by $\mathcal{A}$ corresponds to a path in $G$ of length $n$. Therefore, a Hamiltonian path can exist in $G$ if and only if there exists some word of length $n$ containing each symbol from $\Sigma$ exactly once. In other words, a Hamiltonian path exists in $G$ if and only if $\mathcal{A}$ contains a $1$-universal word. 
	% In the other direction, if a Hamiltonian path exists in $G$, a $1$-universal word exists in $\mathcal{A}$ corresponding to the Hamiltonian path. Similarly, if no such path exists, then no $1$-universal word can exist in $\mathcal{A}$. 
	Hence it is NP-hard to determine if at least one word accepted by $\mathcal{A}$ is $k$-universal, even for $k = 1$.
\end{proof}
\begin{figure}
	\begin{tabular}{c c c}
	\scalebox{0.8}{
	\begin{tikzpicture}[->,>=stealth',shorten >=1pt,auto,node distance=2.8cm,
		semithick]
		%		\tikzstyle{every state}=[draw=none,text=white]
		
		\node[state] (A)                    {$v_1$};
		\node[state] (B) [above right of=A] {$v_2$};
		\node[state] (C) [below right of=B] {$v_3$};
		
		\path (A) edge [bend right] node {} (B)
		edge [bend right] node {} (C)
		(B) edge [bend right] node {} (C)
		edge [bend right] node {} (A)
		(C) edge [bend right] node {} (B);
		\node at (-1,1.5) {$G=(V,E)$};
	\end{tikzpicture}}
	& 
	
	&
	\scalebox{0.7}{
	\begin{tikzpicture}[->,>=stealth',shorten >=1pt,auto,node distance=2.5cm,
		semithick]
		\tikzstyle{every state}=[initial text=$ $]
		
		\node[state] (q11) {$q_{1,1}$};
		\node[state] (q21) [right of=q11] {$q_{2,1}$};
		\node[state,accepting] (q31) [right of=q21] {$q_{3,1}$};
		\node[state] (q12) [below of=q11] {$q_{1,2}$};
		\node[state] (q22) [right of=q12] {$q_{2,2}$};
		\node[state,accepting] (q32) [right of=q22] {$q_{3,2}$};
		\node[state] (q13) [below of=q12] {$q_{1,3}$};
		\node[state] (q23) [right of=q13] {$q_{2,3}$};
		\node[state,accepting] (q33) [right of=q23] {$q_{3,3}$};
		\node[state,initial] (qi) [left of=q12] {$q_0$};
		\node[state] (qf)  [right of=q32] {$q_f$};
		
		\path 
		(q31) edge node {$\mathtt{1,2,3}$} (qf)
		(q32) edge node {$\mathtt{1,2,3}$} (qf)
		(q33) edge [below,right=0.7] node {$\mathtt{1,2,3}$} (qf)
		(q11) [bend left, above] edge node {$\mathtt{2}$} (q22)
		(q21) [bend left, above] edge node {$\mathtt{2}$} (q32)
		(q12) [bend right, below] edge node {$\mathtt{1}$} (q21)
		(q22) [bend right, below] edge node {$\mathtt{1}$} (q31)
		(q12) [bend left, below] edge node {$\mathtt{3}$} (q23)
		(q22) [bend left, above] edge node {$\mathtt{3}$} (q33)
		(q13) [bend right, above] edge node {$\mathtt{2}$} (q22)
		(q23) [bend right, below] edge node {$\mathtt{2}$} (q32)
		(q11) edge [in=-120,out=-70,left=0.2] node {$\mathtt{3}$} (q23)
		(q21) [in=120,out=70,above] edge node {$\mathtt{3}$} (q33)
		(qi) edge [dotted,bend left] node {$\mathtt{1}$} (q11)
		(qi) edge [dotted, in=-180,out=0] node {$\mathtt{2}$} (q12)
		(qi) edge [dotted,bend right] node {$\mathtt{3}$} (q13);
		\node at (-2.5,0) {$\mathcal{A}$};
		\end{tikzpicture}}
	\end{tabular}
	\caption{The constructed automaton $\mathcal{A}$ from the graph $G$ via the reduction from Theorem~\ref{thm:NP_hard_1_universal}.
	% when using the reduction function from Theorem~\ref{thm:NP_hard_1_universal}. 
	%The dotted lines indicate the transitions from $q_0$. 
	We omit the transitions between $q_{i,j}$ and $q_f$, for every $i \in [2], j \in [3]$, for better readability.}
	\label{img:bigautomataexample}
	\end{figure}

\else
\fi

\ifpaper
\bigskip
\noindent
\textbf{Lemma~\ref{lem:making_a_path_longer}.}
    Let $\pi$ be an $(\ell - 1)$-length path in the NFA $\mathcal{A}$ ending at $q$ and corresponding to the word $w_{\pi}$, such that $\iota(w_{\pi}) = c$ and $\letters(\r(w_{\pi})) = \mathcal{R}$. % containing $c$ arches and the set of symbols $\mathcal{R}$ in the post arch suffix.
    Then the word $w_{\pi'}$ corresponding to the path $\pi'$ formed by following a transition labelled $\tx\in\Sigma$ from $q$ either:
    \begin{itemize}
        \item has an empty rest $(\r(w_{\pi'}) = \varepsilon)$ if $\mathcal{R} \cup \{\tx\} = \Sigma$ and hence $\iota(w_{\pi'}) = c + 1$, or% and $\r(w_{p'}) = \varepsilon$, or
        \item has a rest equal to $\mathcal{R} \cup \{ \tx \}$ $(\letters(\r(w_{\pi'})) =  \mathcal{R} \cup \{\tx\})$ if $\mathcal{R} \cup \{\tx\} \subsetneq \Sigma$ and hence $\iota(w_{\pi'}) = c$. % and $\letters(\r(w_{p'})) =  \mathcal{R} \cup \{x\}$. %if $\mathcal{R} \cup \{x\} \neq \Sigma$.
    \end{itemize}
\input{proofs/making_a_path_longer.tex}
\else
\fi

%%% lem:number_of_paths
\ifpaper
	\bigskip
	%Lem25
	\noindent
	\textbf{Lemma~\ref{lem:number_of_paths}.}
    Let $\mathcal{A}$ be a non-deterministic finite automaton and assume that $T[q_0,0,0,\emptyset]$ is given.
    Notice that given $q\in Q$, the combination $(q',\tx)\in Q\times\Sigma$ only contributes to $T[q,\ell,c,\mathcal{R}]$ if we have $q'\in\Delta(q,\tx)$. Thus, we have for all $\ell\geq 1$    
    $$ 
    T[q, \ell, c, \mathcal{R}] =
        \sum\limits_{\overset{\tx \in \Sigma,}{q'\in\Delta(q,\tx)}} \begin{cases}
            0, & \mbox{if }\tx \notin \mathcal{R} \text{ and } \mathcal{R} \neq \emptyset,\\
            0, & \mbox{if }\mathcal{R} = \emptyset, c = 0,\\
            T[q', \ell - 1, c - 1, \Sigma \setminus \{\tx\}], & \mbox{if } \mathcal{R} = \emptyset, c > 0, \\
                T[q', \ell - 1, c, \mathcal{R} \setminus \{\tx\}] 
                + T[q', \ell - 1, c, \mathcal{R}],
                 & \mbox{if }\mathcal{R} \neq \emptyset, x \in \mathcal{R}.
        \end{cases}
    $$
	\input{proofs/number_of_paths.tex}
\else
\fi

%%% col:generally_computing_the_path_table
\ifpaper
	\bigskip
	%Lem26
	\noindent
	\textbf{Corollary~\ref{col:generally_computing_the_path_table}.}
  	We have
  	$U[q,\ell]= \sum{\tx \in \Sigma,q'\in\Delta(q,\tx)}
  	U[q', \ell - 1] + T[q', \ell - 1, k - 1, \Sigma \setminus \{\tx\}]$.
\input{proofs/generally_computing_the_path_table.tex}
\else
\fi

%%% thm:counting_exactly_ell_k_subsequence_universal_words
\ifpaper
	\bigskip
	%Thm27
	\noindent
	\textbf{Theorem~\ref{thm:counting_exactly_ell_k_subsequence_universal_words}.}
    The number of $k$-universal accepting paths of length $m$ of an NFA $\mathcal{A}$ can be computed in $O^*(m^2 n^2 k 2^{\sigma})$ time.
%    $O(m^2 n^2 k \sigma 2^{\sigma})$ time.
	\input{proofs/counting_exactly_ell_k_subsequence_universal_words.tex}
\else
\fi

%%% col:counting_up_to_ell_k_subsequence_univeral_paths
\ifpaper
	\bigskip
	\noindent
	\textbf{Corollary~\ref{col:counting_up_to_ell_k_subsequence_univeral_paths}.}
    The number of  $k$-universal paths of length at most $m$ accepted by an NFA $\mathcal{A}$ with $n$ states can be computed in $O^*(m^2 n^2 k 2^{\sigma})$ time.
    % $O(m^2 n^2 k \sigma 2^{\sigma})$ time.
	\input{proofs/col_counting_up_to_ell_k_subsequence_univeral_paths.tex}
\else
\fi

\ifpaper
\bigskip
\begin{example}\label{example}
Consider again the automaton $\mathcal{A}$ from Figure~\ref{img:universal_automaton}. Let $k=2$. We have $T[q_0,0,0,\emptyset]=1$ and $T[q_0,1,0,\{\ta\}]=T[q_0,1,0,\{\tb\}]=T[q_1,1,0,\{\tc\}]=1$.
For the path of length $2$, we have the words $\ta\ta,\ta\tc,\tb\ta,\tb\tc$, and $\tc\ta$. Thus, we have
\begin{align*}
T[q_0,2,0,\{\ta\}] &=T[q_0,1,0,\emptyset]+T[q_0,1,0,\{a\}]=0+1=1,\\
T[q_0,2,0,\{\ta,\tb\}] &= T[q_0,1,0,\{\tb\}]+T[q_0,1,0,\{\ta,\tb\}]=1+0=1,\\
T[q_1,2,0,\{\tx,\tc\}] &= T[q_0,1,0,\{\tx\}]+T[q_0,1,0,\{\tx,\tc\}]=1+0=1,\forall \tx\in\{\ta,\tb\},\\
T[q_2,2,0,\{\tc,\ta\}] &= T[q_1,1,0,\{\tc\}]+T[q_1,1,0,\{\tc\}]=1+0=1.
\end{align*}
For words of length $3$ and $4$, we get the following values (all others are $0$).
\begin{center}
\begin{tabular}{cccc|c}
$q'$ & $\ell$ & $c$ & $\mathcal{R}$ & amount \\ \hline
$q_0$ & 3& 0 &$\{\ta\}$ & $1$ \\
$q_0$ & 3& 0 &$\{\tb\}$ & $1$ \\
$q_0$ & 3& 0 &$\{\ta,\tb\}$ & $6$ \\
$q_1$ & 3& 0 &$\{\ta,\tc\}$ & $1$ \\
$q_1$ & 3& 0 &$\{\tb,\tc\}$ & $1$ \\
$q_1$ & 3& 1 &$\emptyset$ & $2$ \\
$q_2$ & 3& 1 &$\emptyset$ & $2$ \\
$q_2$ & 3& 0 &$\{\ta,\tc\}$ & $1$ 
\end{tabular}
\hspace{1cm}
\begin{tabular}{cccc|c}
$q'$ & $\ell$ & $c$ & $\mathcal{R}$ & amount \\ \hline
$q_0$ & 4& 0 &$\{\ta\}$ & $1$ \\
$q_0$ & 4& 0 &$\{\tb\}$ & $1$ \\
$q_0$ & 4& 0 &$\{\ta,\tb\}$ & $14$ \\
$q_1$ & 4& 0 &$\{\ta,\tc\}$ & $1$ \\
$q_1$ & 4& 0 &$\{\tb,\tc\}$ & $1$ \\
$q_1$ & 4& 1 &$\emptyset$ & $6$ \\
$q_2$ & 4& 0 &$\{\ta,\tc\}$ & $3$ \\
$q_2$ & 4& 1 &$\{\ta\}$ & $2$ \\
$q_2$ & 4& 1 &$\{\tb\}$ & $2$ \\
$q_2$ & 4& 1 &$\{\tc\}$ & $2$ \\
$q_2$ & 4& 1 &$\emptyset$ & $3$
\end{tabular}
\end{center}
\end{example}
\fi

%%% lem:reaching_every_state_further
%\ifpaper
%\bigskip
%\noindent
%\textbf{Lemma~\ref{lem:reaching_every_state_further}.}
%   Given a pair of states $q, q' \in Q$ in the automaton $\mathcal{A}$ such that there exists a path $P$ from $q$ to $q'$ where the final transition in $P$ is labelled $\tx \in \Sigma$.
%   Then, there exists some path $P'$ of length at most $n$ from $q$ to $q'$ where the final transition in the path is labelled $\tx$.
%\input{proofs/reaching_every_state_further.tex}
%\else
%\fi

%%% lem:ksu_min_length
%\ifpaper
%\bigskip
%Lem37
%\noindent
%\textbf{Lemma~\ref{lem:ksu_min_length}.}
%  Given an automaton $\mathcal{A}$, the shortest $k$-subsequence universal word recognised by $\mathcal{A}$ must have length at most $k n \sigma$.
%\input{proofs/ksu_min_length.tex}
%\else
%\fi

%%% thm:counting_everything

\ifpaper
\bigskip
	\noindent
	\textbf{Theorem~\ref{thm:counting_everything}.}
    The total number of $k$-universal words (resp., paths) accepted by a DFA (resp., NFA) $\mathcal{A}$ can be determined in 
    $O^*(n^4 k^2 2^{\sigma})$ time (resp.,  $O^*(n^4 k^3 2^{\sigma})$ time),
    % $O(n^4 k^2 \sigma^2 2^{\sigma})$ time (resp.,  $O(n^4 k^3 \sigma^3 2^{\sigma})$ time),
   for $k\leq n$. For $k\geq n$, this number is either $0$ or $\infty$, and can be determined in
     $O^*(n^3 2^\sigma)$ time. 
	\input{proofs/counting_everything.tex}
\else
\fi

%%% thm:solving_existance
%\ifpaper
%\bigskip
%\noindent
%\textbf{Theorem ~\ref{thm:solving_existance}.}
%$k$-ASUPFA can be solved for an $n$ state automaton $\mathcal{A}$ in $O(n^3 k \sigma 2^{\sigma})$ time.
%\ifpaper
%\input{proofs/solving_existance.tex}
%\else
%\fi

%%% thm:ESUPFA_solving
%\ifpaper
%\bigskip
%\noindent
%\textbf{Theorem~\ref{thm:ESUPFA_solving}.}
%  $k$-ESUPFA can be solved for an automaton $\mathcal{A}$ with $n$ states and an alphabet of size $\sigma$ in $O(n^3 k^2 \sigma^2 2^{\sigma})$ time.
%\ifpaper
%\input{proofs/ESUPFA_solving.tex}
%\else
%\fi

%%% thm:ranking_fixed_length
\ifpaper

	\bigskip
	\noindent
	\textbf{Theorem~\ref{thm:ranking_fixed_length}.}
    The rank $w \in \Univ_{\mathcal{A}_m, k}$ 
    can be determined in $O^*(m^2 n^2 k 2^{\sigma})$ time.
    % can be determined in $O(m^2 n^2 k \sigma 2^{\sigma})$ time.
    
	\input{proofs/ranking_fixed_length.tex}
\else	
\fi

%%% col:ranking_up_to_k_length
\ifpaper
\bigskip
\noindent
\textbf{Corollary~\ref{col:ranking_up_to_k_length}.}
    The rank of $w\in \Univ_{\mathcal{A}_{\leq m}, k}$
    can be determined in % $O(m^2 n^2 k \sigma 2^{\sigma})$ time.
    $O^*(m^2 n^2 k 2^{\sigma})$ time.
\input{proofs/ranking_up_to_k_length.tex}
\else
\fi

%%% col:ranking_everything
\ifpaper
\bigskip
\noindent
\textbf{Corollary~\ref{col:ranking_everything}.}
    The rank of $w \in \Univ_{L(\mathcal{A}), k}$ can be determined in % $O(n^4 k^3 \sigma^3 2^{\sigma})$ time.
    $O^*(n^4 k^3 2^{\sigma})$ time.
	\input{proofs/ranking_everything.tex}
\else
\fi
